# Supplementary material for: Inner Skin Effects on Non-Hermitian Topological Fractals
Source: arXiv:2202.07658 ancillary file (2023-01-17)
Supplement: Supplementary file 1 [file SupplementaryInformation_NHFractal.pdf]

# Supplemental Information: Inner Skin Effects on Non-Hermitian Topological Fractals

Sourav Manna[1] and Bitan Roy[2]
[1]Department of Condensed Matter Physics, Weizmann Institute of Science, Rehovot 7610001, Israel
[2]Department of Physics, Lehigh University, Bethlehem, Pennsylvania, 18015, USA
(Dated: November 5, 2022)

The Supplemental Information (SI) contains derivation of the real space Hamiltonian for (a) non-Hermitian (NH) Chern insulator [Supplementary Note 1], (b) NH second-order topological insulator [Supplementary Note 2], (c) NH first-order topological superconductor [Supplementary Note 3], (d) NH second-order topological superconductor [Supplementary Note 4], and (e) additional numerical results [Supplementary Note 5 and Supplementary Figure 1-Supplementary Figure 12].

## Supplementary Note 1. NH CHERN INSULATOR MODEL IN REAL SPACE

The model for a two-dimensional (2D) Chern insulator, defined on a square lattice is captured by the spinless Bernevig-Hughes-Zhang model [1], given by

$$\hat{h}_{\rm CI} = t\left[\sin(k_x a)\tau_1 + \sin(k_y a)\tau_2\right] + \left[-m_0 + t_0\left\{\cos(k_x a) + \cos(k_y a)\right\}\right]\tau_3, \tag{S1}$$

where $a$ is the lattice spacing, which can be set to unity. The Pauli matrices $\tau_{1,2,3}$ operate on the orbital indices, and $\boldsymbol{k} = (k_x, k_y)$ is the spatial momenta. We seek to implement this model on an arbitrary 2D lattice system, which besides the square lattice also includes quasicrystals, amorphous network and Sierpinski carpet fractal lattice. For this purpose, associated to each momentum dependent form factors, we identify the term defined on real space, both of which transform identically under the pertinent symmetry operations. They are (a) four-fold rotational symmetry, (b) reflection symmetry about $x$ axis, and (c) reflection symmetry about the $y$ axis. Such symmetry analyses on momentum and real spaces are shown in Supplementary Table 1. We then arrive at the model for the real space 2D Chern insulator

$$\hat{h}_0 = \sum_{j \neq k} \frac{F(r_{jk})}{2}\left[-it(\cos\phi_{jk}\tau_1 + \sin\phi_{jk}\tau_2) + t_0\Gamma_3\right] - \sum_j \left[m_0\tau_3\right]. \tag{S2}$$

In the last step we augment each hopping amplitude by a rotationally symmetric function $F(r_{jk}) = \Theta(r_{jk} - R)\exp\left[1 - r_{jk}/r_0\right]$ such that the sites remain well connected, especially in the absence of translational symmetry. As

| Symmetry analyses in Brillouin zone (BZ) | | | | | Symmetry analyses in real space (RS) | | | | |
|---|---|---|---|---|---|---|---|---|---|
| Function | $R^{\rm BZ}_{\pi/2}$ | $R^{\rm BZ}_x$ | $R^{\rm BZ}_y$ | $\mathcal{K}$ | Function | $R^{\rm RS}_{\pi/2}$ | $R^{\rm RS}_x$ | $R^{\rm RS}_y$ | $\mathcal{K}$ |
| $\sin k_x$ | $-\sin k_y$ | $\sin k_x$ | $-\sin k_x$ | - | $i\cos\phi_{jk}$ | $-i\sin\phi_{jk}$ | $i\cos\phi_{jk}$ | $-i\cos\phi_{jk}$ | - |
| $\sin k_y$ | $\sin k_x$ | $-\sin k_y$ | $\sin k_y$ | - | $i\sin\phi_{jk}$ | $i\cos\phi_{jk}$ | $-i\sin\phi_{jk}$ | $i\sin\phi_{jk}$ | - |
| $\cos k_x + \cos k_y$ | $\cos k_x + \cos k_y$ | $\cos k_x + \cos k_y$ | $\cos k_x + \cos k_y$ | + | $C$ | $C$ | $C$ | $C$ | + |
| $m_0$ | $m_0$ | $m_0$ | $m_0$ | + | $m_0$ | $m_0$ | $m_0$ | $m_0$ | + |
| $\cos k_x - \cos k_y$ | $-(\cos k_x - \cos k_y)$ | $\cos k_x - \cos k_y$ | $\cos k_x - \cos k_y$ | + | $\cos 2\phi_{jk}$ | $-\cos 2\phi_{jk}$ | $\cos 2\phi_{jk}$ | $\cos 2\phi_{jk}$ | + |

Supplementary Table 1: Symmetry analyses of various terms appearing in the momentum space (first five columns) and real sapce (last five columns) Hamiltonian [2]. Terms transforming identically under symmetry transformations appear in the same row. Here $R^{\rm BZ}_{\pi/2}$ represents a rotation by $\pi/2$ about the $z$ direction under which $\boldsymbol{k} \to (-k_y, k_x)$, while $R^{\rm BZ}_x$ corresponds to reflection about the $x$ axis under which $\boldsymbol{k} \to (k_x, -k_y)$, and finally $R^{\rm BZ}_y$ stands for reflection about the $y$ axis under which $\boldsymbol{k} \to (-k_x, k_y)$. On the other hand, $R^{\rm RS}_{\pi/2}$ represents a rotation by $\pi/2$ about the $z$ direction in the real space under which $\phi_{jk} \to \phi_{jk} + \pi/2$, $R^{\rm RS}_x$ corresponds to reflection about the $x$ axis in the real space under which $\phi_{jk} \to 2\pi - \phi_{jk}$, and $R^{\rm RS}_y$ corresponds to reflection about the $y$ axis in the real space under which $\phi_{jk} \to \pi - \phi_{jk}$. Here $m_0$ and $C$ are *real* constants, $\boldsymbol{k} = (k_x, k_y)$ is the momentum, and $\phi_{jk}$ is the azimuthal angle between sites $j$ and $k$, measured about the horizontal direction. We also summarize the transformation of each term under complex conjugation ($\mathcal{K}$), with $\mathcal{K}\boldsymbol{k} \to -\boldsymbol{k}$. In the fifth and tenth columns $+(-)$ corresponds to even (odd).

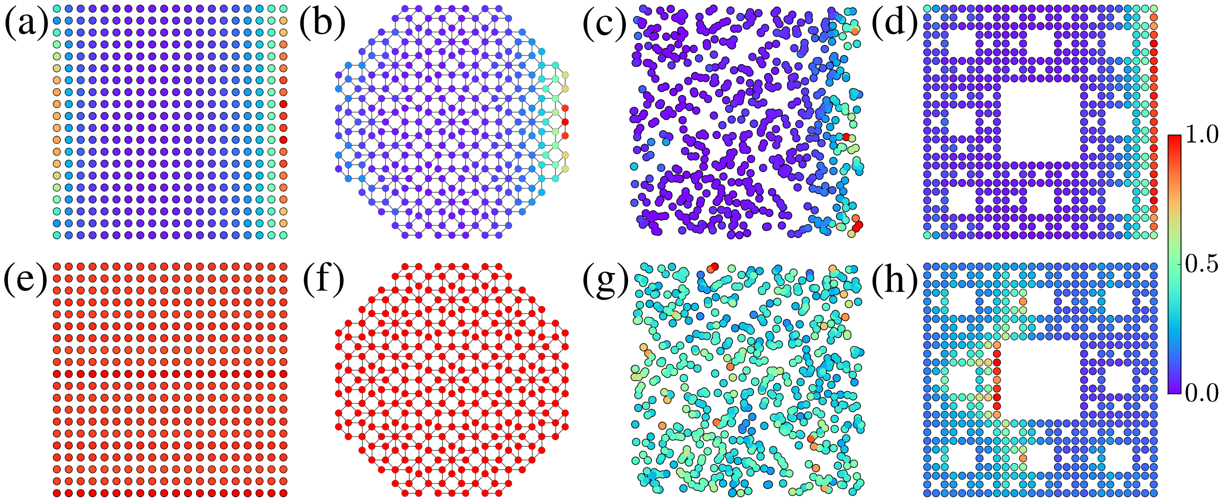


Supplementary Figure 1: Total normalized weight of all the right eigenvectors of $H_{\rm FO}$ on (a) square lattice, (b) Ammann-Beenker quasicrystal, (c) amorphous network and (d) Sierpinski carpet fractal lattice of third generation with open boundary condition for $m_0 = 0$ and $\boldsymbol{h} = (0.4, 0, 0)$ [panels (a), (c) and (d)], $m_0 = 1.0$ and $\boldsymbol{h} = (0.75, 0, 0)$ [panel (b)], and $R = 2a$ [panels (a), (b) and (d)]. Throughout we set $t = t_0 = 1$ and $r_0 = a$. In panel (c) $R = 0.98a$, where $a$ is the linear dimension of the system in both $x$ and $y$ directions. In (a) and (d), $a$ is the nearest-neighbor distance, and $a$ is the length of all the arms in panel (b). Top panel shows skin effect at the outer right edges of these systems. Panels (e), (f), (g) and (h) are same as panels (a), (b), (c) and (d), respectively, but with periodic boundary condition (PBC) only in the $x$ direction. The lower panel shows that skin effect is present only at the inner edges of the Sierpinski carpet fractal with PBC, while it is absent in other lattice systems with PBC. Results in panels (e)-(f) remain qualitatively unchanged with additional PBC in the $y$ direction.

all the non-Hermitian (NH) terms are momentum independent or on site quantities, they can be directly implemented on any real space lattice system. Finally, upon introducing an appropriate two-component spinor $c_j = [c_{j\alpha}, c_{j\beta}]^\top$, $c_{j\alpha}$ is the fermionic annihilation operator at site $j$ and on orbital $\alpha$, we arrive at the real space model for the NH 2D Chern insulator, given by

$$H_{\rm FO} = \sum_{j \neq k} \frac{F(r_{jk})}{2} c_j^\dagger \big[ -it(\cos\phi_{jk}\tau_1 + \sin\phi_{jk}\tau_2) + t_0\tau_3 \big] c_k - \sum_j c_j^\dagger \big[ m_0 \Gamma_3 \big] c_j + i\, c_j^\dagger \big[ h_x\tau_1 + h_y\tau_2 + h_z\tau_3 \big] c_j, \tag{S3}$$

which is identical to Eq. (1) of the main text.

## Supplementary Note 2. NH HIGHER-ORDER INSULATOR MODEL IN REAL SPACE

The Hamiltonian for a 2D second-order topological insulator, defined on a square lattice is described by the Benalcazar-Bernevig-Hughes (BBH) model [3], given by

$$\hat{h}_{\rm BBH} = t \left[ \sin(k_x a)\tilde{\Gamma}_1 + \sin(k_y a)\tilde{\Gamma}_2 \right] + \left[ -\tilde{m}_0 + t_2\cos(k_x a) \right] \tilde{\Gamma}_3 + \left[ -\tilde{m}_0 + t_2 \cos(k_y a) \right] \tilde{\Gamma}_4, \tag{S4}$$

where $\tilde{\Gamma}_\mu$ are four-dimensional mutually anticommuting Hermitian matrices, with $\mu = 1, 2, 3, 4$. This model can also be written as

$$\begin{aligned} \hat{h}_{\rm BBH} &= t \left[ \sin(k_x a)\tilde{\Gamma}_1 + \sin(k_y a)\tilde{\Gamma}_2 \right] + \left[ -2\tilde{m}_0 + t_2 \{ \cos(k_x a) + \cos(k_y a) \} \right] \left( \frac{\tilde{\Gamma}_3 + \tilde{\Gamma}_4}{2} \right) \\ &+ t_2 \left[ \{ \cos(k_x a) - \cos(k_y a) \} \right] \left( \frac{\tilde{\Gamma}_3 - \tilde{\Gamma}_4}{2} \right). \end{aligned} \tag{S5}$$

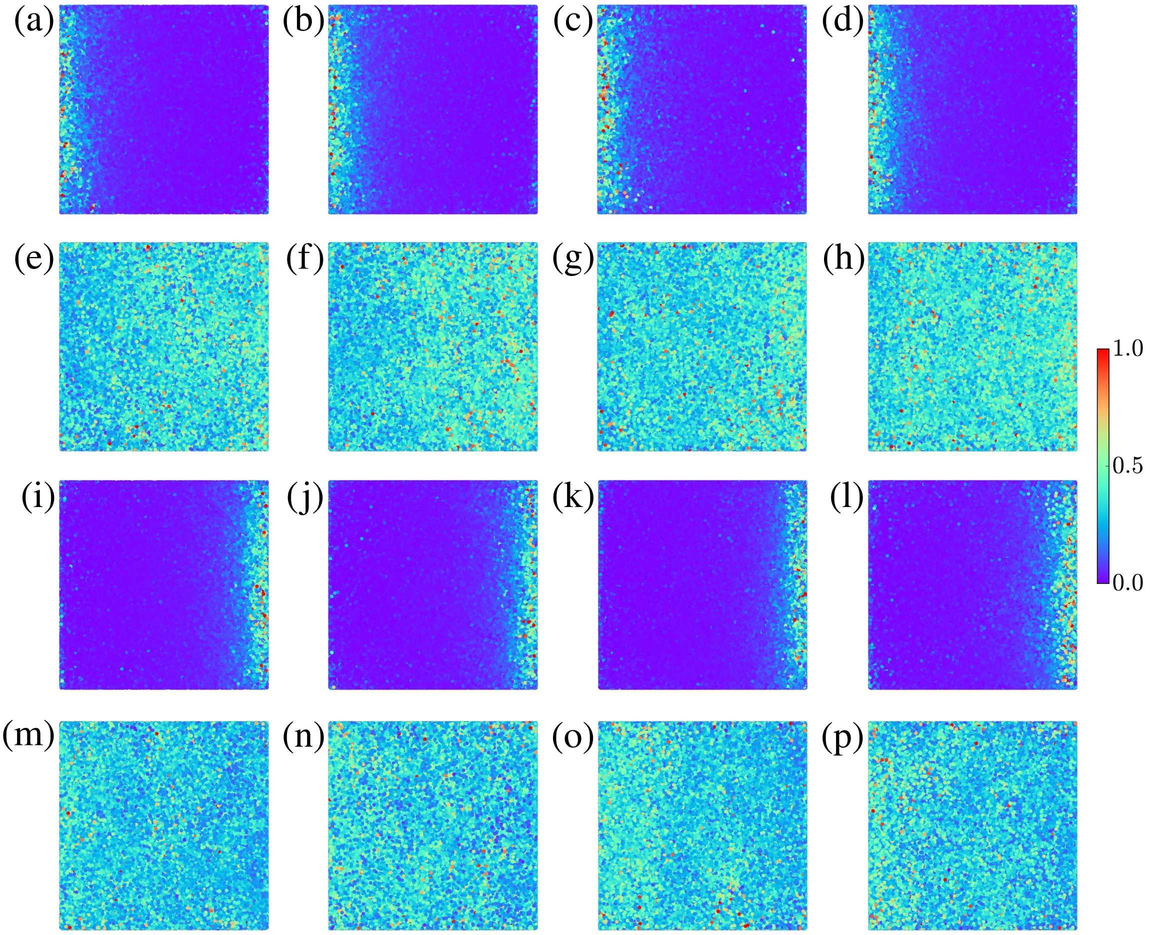


Supplementary Figure 2: Total (normalized by its maximum value) density of all the left (first and second rows) and right (third and fourth rows) eigenvectors, with open (first and third rows) and periodic (second and fourth) boundary conditions, computed after 250 (first column), 500 (second column), 750 (third column) and 1000 (fourth column) random and independent realizations of 600 lattice sites, constituting the amorphous network. While the left (right) eigenvectors show skin effect on the left (right) edge of the amorphous network with open boundary condition, the density distribution of left or right eigenvectors becomes gradually more smooth with increasing number of disorder realizations when we impose periodic boundary condition in the $x$ direction of the amorphous network. Results in the second and fourth rows remain qualitatively unchanged with additional periodic boundary condition in the $y$ direction. For numerical simulation we throughout take $t = t_0 = m_0 = 1$, $h_x = 0.4$, $R = 2a$ and $r_0 = a$ in $H_{\rm FO}$. Here $a$ is the linear dimension of the amorphous network in both $x$ and $y$ directions.

The last form of $\hat{h}_{\rm BBH}$ conforms to the following alternative representation of the Hamiltonian for a 2D second-order topological insulator

$$\hat{h}_{\rm SO} = t\left[\sin(k_x a)\Gamma_1 + \sin(k_y a)\Gamma_2\right] + \left[-m_0 + t_0\{\cos(k_x a) + \cos(k_y a)\}\right]\Gamma_3 + g\left[\{\cos(k_x a) - \cos(k_y a)\}\right]\Gamma_4, \tag{S6}$$

with the following correspondences among various parameters and matrices appearing in $\hat{h}_{\rm BBH}$ and $\hat{h}_{\rm SO}$ [4]

$$\Gamma_1 = \tilde{\Gamma}_1,\ \Gamma_2 = \tilde{\Gamma}_2,\ \Gamma_3 = \left(\frac{\tilde{\Gamma}_3 + \tilde{\Gamma}_4}{2}\right),\ \Gamma_4 = \left(\frac{\tilde{\Gamma}_3 - \tilde{\Gamma}_4}{2}\right),\ m_0 = 2\tilde{m}_0,\ t_0 = t_2,\ g = t_2. \tag{S7}$$

Note that $\Gamma_\mu$ constitute yet another set of four mutually anticommuting four-dimensional Hermitian matrices, with $\mu = 1, 2, 3, 4$. The real space version of the Hamiltonian $\hat{h}_{\rm SO}$ can now be derived by following the same methodology discussed in Supplementary Note 1 upon consulting the symmetry analyses summarized in Supplementary Table 1. In the basis of a four-component spinor $c_j = [c_{j\uparrow\alpha}, c_{j\uparrow\beta}, c_{j\downarrow\alpha}, c_{j\downarrow\beta}]^\top$, where $c_{j\sigma\alpha}$ is the fermionic annihilation operator

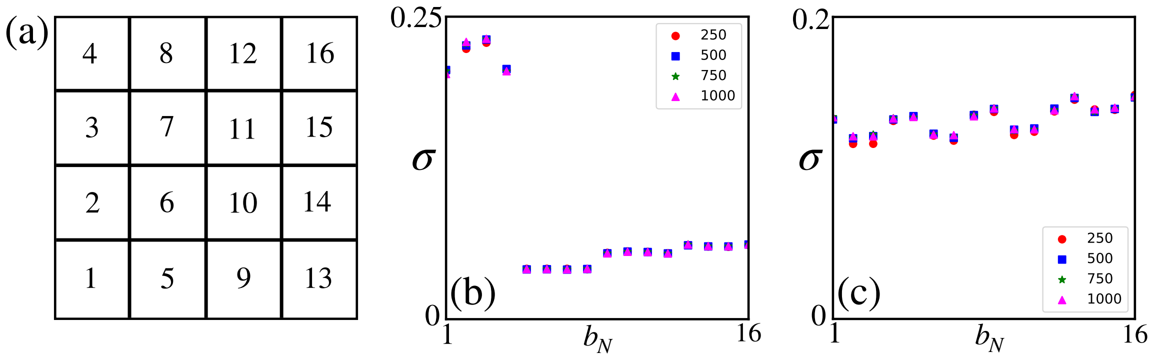


Supplementary Figure 3: (a) Assignment of the bin number ($b_N$) of an amorpous network split into sixteen bins. (b) Standard deviation ($\sigma$) of the average density of all the left eigenvectors on each bin, computed with respect to its average density in the whole system [see Eq. (S16)] with open boundary condition, showing non-Hermitian skin effect at the left edge of the system (bin number 1-4). (c) The same quantity with periodic boundary condition, showing (almost) uniform distribution of the weight of the left eigenvector, thus absence of any skin effect. We compute this quantity for 250, 500, 750 and 1000 realizations of 600 sites, distributed randomly and independently. Data in panels (b) and (c) are generated from Supplementary Figure 2. The conclusions remain qualitatively unchanged for the right eigenvectors (not shown here explicitly), except the skin effect shows up in bins 13-16.

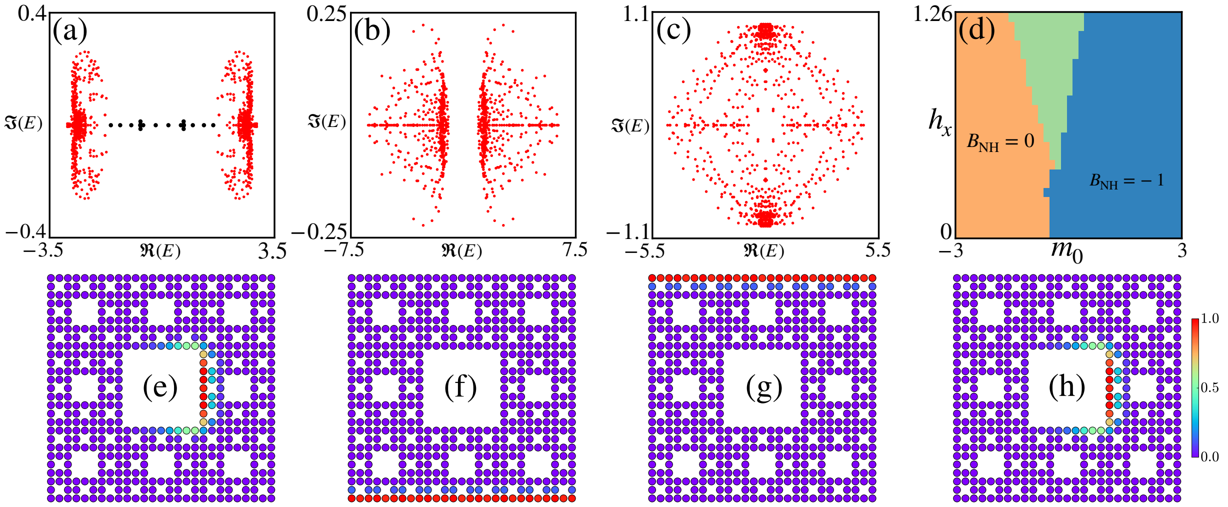


Supplementary Figure 4: Energy spectra of $H_{\rm FO}$ on Sierpinski carpet fractal lattice of third generation with periodic boundary conditions (PBCs) in $x$ and $y$ directions for (a) $m_0 = 2.0$ and $h_x = 0.5$, (b) $m_0 = -2.0$ and $h_x = 0.4$ and (c) $m_0 = -0.5$ and $h_x = 1.0$. Throughout we set $t = t_0 = 1$, $r_0 = a$, $R = 2a$. In (a) and (b) the spectra show line gap, while only in (a) there exist topological modes (black dots) residing on the inner edges of the fractal lattice. In (c) the spectra display point gap. The non-Hermitian Bott index $B_{\rm NH} = -1$ in (a), yielding a NH Chern insulator [blue region in (d)]. In (b) $B_{\rm NH} = 0$, representing a trivial insulator [orange region in (d)]. However, in (c) the $B_{\rm NH}$ is not well defined [green region in (d)]. (d) Phase diagram in the $(m_0, h_x)$ plane, hosting these three phases. Joint density of the left eigenvectors of $H_{\rm FO}$ with PBCs only in the $x$ direction for the states with (e) $\Im(E) = 0$ and $\Re(E) = \pm 0.2$, (f) $\Im(E) = 0.5$ and $\Re(E) = 0$, and (g) $\Im(E) = -0.5$ and $\Re(E) = 0.0$. These states are shown in black [(e)] and blue [(f) and (g)] in panel (a) of Fig. 3 of main manuscript. Therefore, these states are localized at inner left [(e)] or outer bottom [(f)] or outer top [(g)] edge. (h) Joint density of the left eigenvectors of of $H_{\rm FO}$ with periodic boundary conditions in the $x$ and $y$ directions for states with $\Im(E) = 0$ and $\Re(E) = \pm 0.2$ [black dots in panel (a)], which is localized at the inner left edge. The corresponding right eigenvectors are localized at the opposite edges. In panel (e)-(h) we normalize density by its maximum value. All the other states shown in black or blue in Fig. 3(a) of main manuscript, or in black in panel (a) of this figure show analogous localization at the inner or outer edges.

at site $j$, with spin projection $\sigma = \uparrow, \downarrow$ and on orbital $\alpha$, the Hamiltonian for a second-order topological insulator in

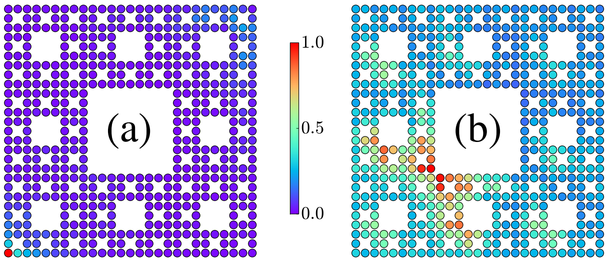


Supplementary Figure 5: The total (normalized) weight of all the right eigenvectors of $H_{\rm SO}$ on a Sierpinski carpet fractal lattices with (a) open and (b) periodic boundary conditions in both $x$ and $y$ directions with $m_0 = 1.5$, $g = 0.5$, $\boldsymbol{h} = (0.35, 0.35, 0)$, $t = t_0 = 1$, $R = 2a$ and $r_0 = a$. Panel (a) shows conventional second-order skin effect at an outer corner, while panel (b) depicts inner second-order skin effect around inner corners of the fractal lattice with open and periodic boundary conditions, respectively.

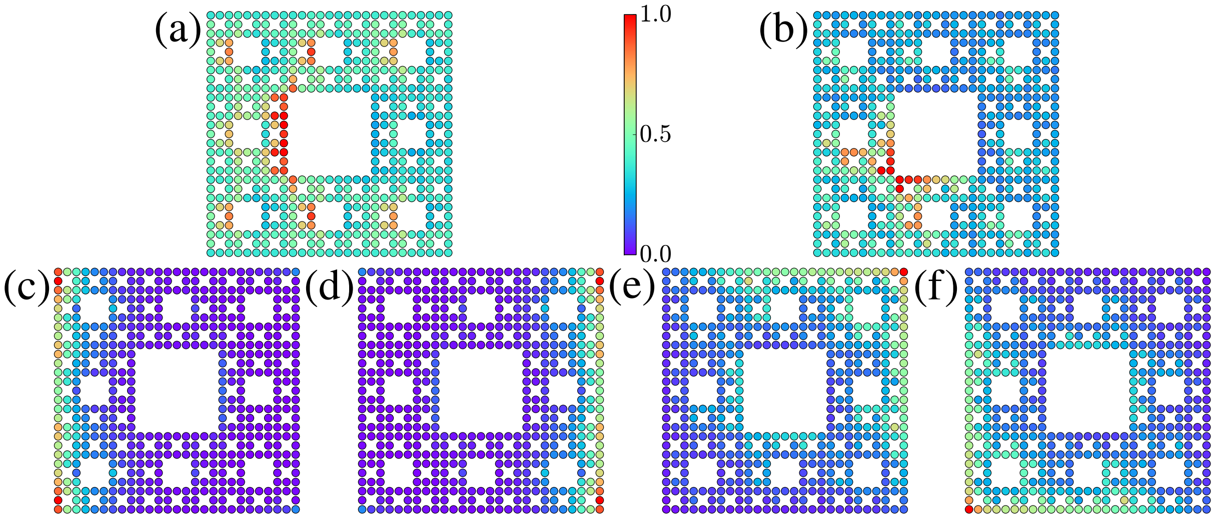


Supplementary Figure 6: Total weight (normalized) of all the right eigenvectors of (a) $H^{\rm pair}_{\rm FO}$ and (b) $H^{\rm pair}_{\rm SO}$ on Siperpinski carpet fractal with periodic boundary condition in (a) $x$ direction and (b) $x$ and $y$ directions. Panels (a) and (b) respectively show inner first-order and second-order skin effects of neutral Majorana fermions at the inner edges and corners. Total weight (normalized) of all the left [panels (c) and (e)] and right [panels (d) and (f)] eigenvectors of $H^{\rm pair}_{\rm FO}$ [panels (c) and (d)] and $H^{\rm pair}_{\rm SO}$ [panels (e) and (f)] on Sierpinski carpet fractal lattices with open boundary conditions. Here we set $m_0 = 0.0$, $\Delta_{\rm FO} = 0.01$ and $\boldsymbol{h} = (0.75, 0, 0)$ [panels (a), (c) and (d)], and $m_0 = 3.0$, $g = 0.5$, $\Delta_{\rm SO} = 0.025$ and $\boldsymbol{h} = (-0.53, -0.53, 0)$ [panels (b), (e) and (f)]. Throughout we set $t = t_0 = 1$, $R = 8a$ and $r_0 = a$. Panels (c) and (d) show conventional first-order Majorana skin effects respectively at the outer left and right edges of the Sierpinski carpet fractals, while panel (e) and (f) depict conventional second-order Majorana skin effects respectively at the outer top-right and bottom-left corners of this system, respectively.

the presence of generic momentum independent or on site NH coupling reads as

$$
\begin{aligned}
H_{\rm SO} \;=\; & \sum_{j \neq k} \frac{F(r_{jk})}{2} c_j^\dagger \big[ -it(\cos\phi_{jk}\Gamma_1 + \sin\phi_{jk}\Gamma_2) + t_0 \Gamma_3 \big] c_k - \sum_j c_j^\dagger \big[ m_0 \Gamma_3 \big] c_j + g \sum_{j\neq k} \frac{F(r_{jk})}{2} c_j^\dagger \Big[ \cos(2\phi_{jk})\, \Gamma_4 \Big] c_k \\
& + \; i\, c_j^\dagger \big[ h_x \Gamma_1 + h_y \Gamma_2 + h_z \Gamma_3 \big] c_j, \qquad \text{(S8)}
\end{aligned}
$$

which is identical to Eq. (4) of the main text. Notice that the one-to-one correspondence between two equivalent representations of a second-order topological insulator in two dimensions, namely $\hat{h}_{\rm BBH}$ and $\hat{h}_{\rm SO}$, does not depend on the representations of the two sets of mutually anticommuting matices $\tilde{\Gamma}_\mu$ and $\Gamma_\mu$, where $\mu = 1, 2, 3, 4$.

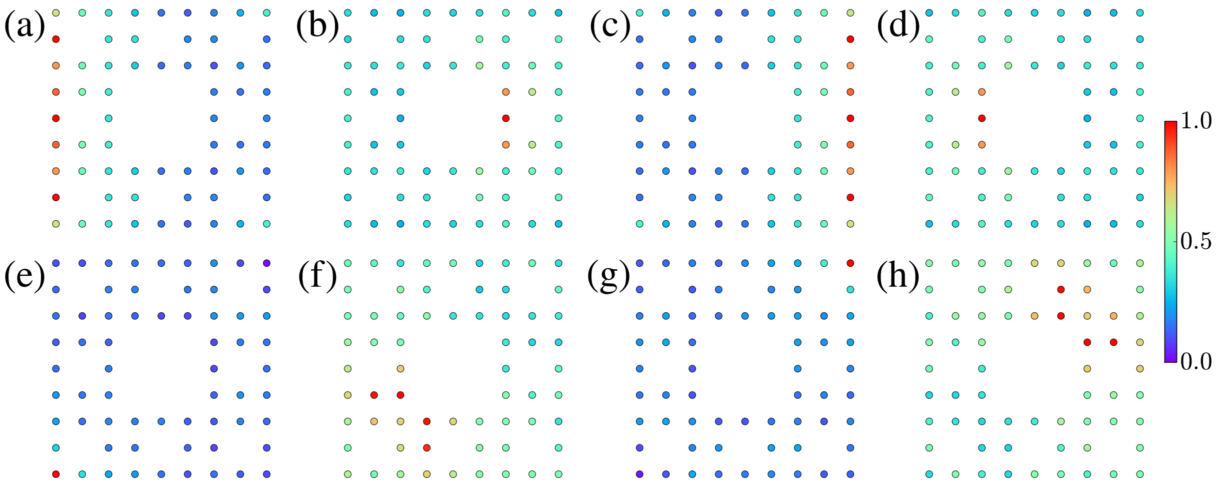


Supplementary Figure 7: Total normalized weight of all the left [panels (a), (b), (e) and (f)] and right [panels (c), (d), (g) and (h)] eigenvectors of $H_{\rm FO}$ [panels (a)-(d)] and $H_{\rm SO}$ [panels (e)-(h)] with open [panels (a), (c), (e) and (g)] and periodic [panels (b), (d), (f) and (h)] conditions, showing conventional first-order [panels (a) and (c)] and second-order [panels (e) and (g)] skin effects, respectively at the outer edge and corner, and inner first-order [panels (b) and (d)] and inner second-order [panels (f) and (h)] skin effects near inner edges and corners, respectively, of the Sierpinski carpet of second generation, containing 64 lattice sites. Throughout we take $t = t_0 = 1$, $R = 2a$ and $r_0 = a$. In the top row we set $m_0 = 0.0$, $\boldsymbol{h} = (0.4, 0, 0)$. In the bottom row we set $m_0 = 1.5$, $g = 0.5$ and $\boldsymbol{h} = (0.35, 0.35, 0)$.

## Supplementary Note 3. NH FIRST-ORDER TOPOLOGICAL SUPERCONDUCTOR MODEL

We devote this section to disclose some key details related to the first-order topological superconductivity and the resulting first-order NH skin effect. For this purpose, we first Nambu double the momentum space Hamiltonian for 2D Chern insulator model from Eq. (S1) in the presence of generic momentum independent NH coupling, leading to

$$\hat{h}^{\rm Nambu}_{CI} = \eta_0 \left[\hat{h}_{\rm CI}\right] + i \left[\eta_3 \tau_1 h_x + \eta_3 \tau_2 h_y + \eta_0 \tau_3 h_z\right], \tag{S9}$$

after absorbing $\tau_1$ matrix in the Nambu or hole part. The newly introduced set of Pauli matrices $\{\eta_\mu\}$ operates on the Nambu or particle-hole index, with $\mu = 0, 1, 2, 3$. In this basis only local or on site pairing is captured by the following effective single-particle Hamiltonian

$$\hat{h}^{\rm pair}_{\rm FO} = \Delta_{\rm FO} \left(\eta_1 \cos\phi + \eta_2 \sin\phi\right) \tau_3, \tag{S10}$$

where $\Delta_{\rm FO}$ is the (real) pairing amplitude and $\phi$ is the U(1) superconducting phase. Without any loss of generality we pick $\phi = 0$ for our numerical analyses. We then follow the procedure summarized in Supplementary Note 1 to arrive at the real space version of the Hamiltonian for a first-order topological pairing in a parent NH system (constituting the normal state)

$$\begin{aligned} H^{\rm pair}_{\rm FO} \;=\; & \sum_{j\neq k} \frac{F(r_{jk})}{2} c^\dagger_j \big[ -it \left(\cos\phi_{jk}\; \eta_0\tau_1 + \sin\phi_{jk}\; \eta_0\tau_2\right) + t_0\; \eta_0\tau_3 \big] c_k - \sum_j c^\dagger_j \big[m_0\; \eta_0\tau_3\big] c_j + \Delta_{\rm FO} \sum_j c^\dagger_j \eta_1 \tau_3 c_j \\ & +\; i \sum_j c^\dagger_j \left[\eta_3\tau_1 h_x + \eta_3 \tau_2 h_y + \eta_0 \tau_3 h_z\right] c_j, \end{aligned} \tag{S11}$$

which is the Nambu doubled version of Eq. (6) of the main text. Here the four-component Nambu doubled spinor is $c_j = \left[c_{j\alpha}, c_{j\beta}, c^\dagger_{j\beta}, c^\dagger_{j\alpha}\right]$. We numerically diagonalize this Hamiltonian to arrive at the conclusions, presented in the main text and this Supplementary Information. For $h_z = 0$, the exact particle-hole symmetry of this model is generated by $\Theta^{\rm pair}_{\rm FO} = \eta_0 \tau_1 {\rm I}_{\mathcal{A}} \mathcal{K}$, where ${\rm I}_{\mathcal{A}}$ is a $\mathcal{A}$-dimensional identity matrix, $\mathcal{A}$ is the total number of lattice sites in the system and $\mathcal{K}$ is the complex conjugation.

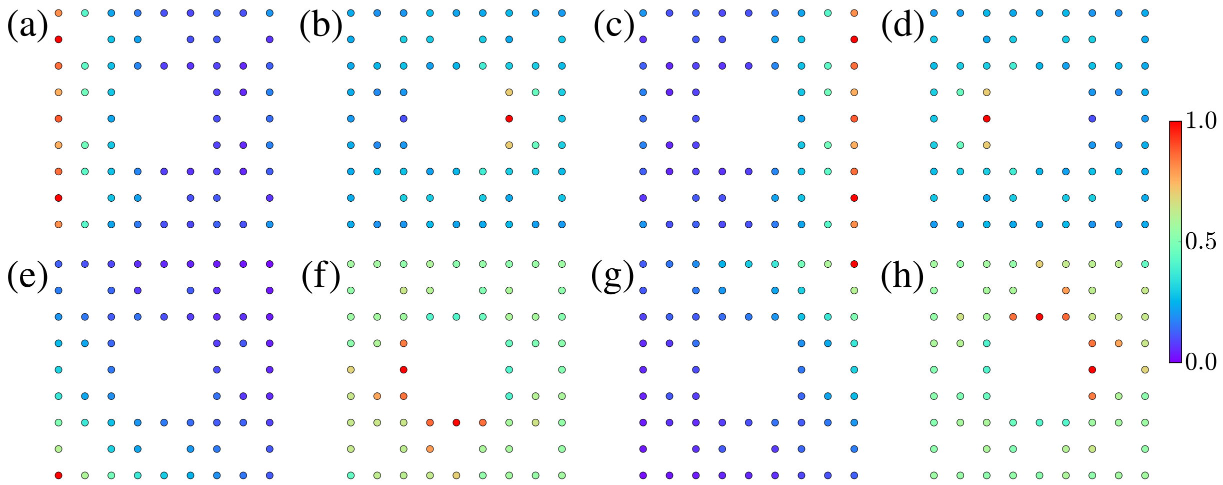


Supplementary Figure 8: Total normalized weight of all the left [panels (a), (b), (e) and (f)] and right [panels (c), (d), (g) and (h)] eigenvectors of $H^{\rm pair}_{\rm FO}$ [panels (a)-(d)] and $H^{\rm pair}_{\rm SO}$ [panels (e)-(h)] with open [panels (a), (c), (e) and (g)] and periodic [panels (b), (d), (f) and (h)] conditions, showing conventional first-order [panels (a) and (c)] and second-order [panels (e) and (g)] skin effects for neutral Majorana fermions, respectively at the outer edge and corner, and inner Majorana first-order [panels (b) and (d)] and inner Majorana second-order [panels (f) and (h)] skin effects near inner edges and corners, respectively, of the Sierpinski carpet of second generation, containing 64 lattice sites. Throughout we take $t = t_0 = 1$, $R = 2a$ and $r_0 = a$. In the top row we set $m_0 = 0.0$, $\Delta_{\rm FO} = 0.01$ and $\boldsymbol{h} = (0.75, 0, 0)$. In the bottom row we set $m_0 = 3.0$, $g = 0.5$, $\Delta_{\rm SO} = 0.025$ and $\boldsymbol{h} = (-0.53, -0.53, 0)$.

## Supplementary Note 4. NH SECOND-ORDER TOPOLOGICAL SUPERCONDUCTOR MODEL

In this section we provide key details related to a second-order topological superconductivity and the resulting second-order NH skin effect. Once again, we Nambu double the corresponding normal state Hamiltonian $\hat{h}_{\rm SO}$ [see Eq. (S6)] in the presence of NH operators, leading to

$$\begin{aligned} \hat{h}^{\rm Nambu}_{\rm SO} &= t\left[\sin(k_x a)\eta_3\Gamma_1 + \sin(k_y a)\eta_3\Gamma_2\right] + \left[-m_0 + t_0\{\cos(k_x a) + \cos(k_y a)\}\right]\eta_3\Gamma_3 \\ &+ g\left[\{\cos(k_x a) - \cos(k_y a)\}\right]\eta_0\Gamma_4 + i\left[\eta_0\Gamma_1 h_x + \eta_0\Gamma_2 h_y + \eta_3\Gamma_3 h_z\right], \end{aligned} \tag{S12}$$

after absorbing $\sigma_2\tau_0$ in the Nambu or hole part. Here the four-component mutually anticommuting Hermitian $\Gamma$ matrices belong to the representation $\Gamma_1 = \sigma_3\tau_1$, $\Gamma_2 = \sigma_0\tau_2$, $\Gamma_3 = \sigma_0\tau_3$ and $\Gamma_4 = \sigma_1\tau_1$. The effective single-particle Hamiltonian for the second-order topological pairing with real amplitude $\Delta_{\rm SO}$ takes the form [5]

$$\hat{h}^{\rm pair}_{\rm SO} = \Delta_{\rm SO}\left(\eta_1\cos\phi + \eta_2\sin\phi\right)\sigma_1\tau_2. \tag{S13}$$

Hereafter we set the U(1) superconducting phase $\phi = 0$. Subsequently, we apply the methodology discussed in Supplementary Note 1 to arrive at the following real space Hamiltonian for the NH second-order topological superconductor

$$\begin{aligned} H^{\rm pair}_{\rm SO} &= \sum_{j\neq k}\frac{F(r_{jk})}{2}c_j^\dagger\left[-it\left(\cos\phi_{jk}\,\eta_3\Gamma_1 + \sin\phi_{jk}\,\eta_3\Gamma_2\right) + t_0\,\eta_3\Gamma_3\right]c_k - \sum_j c_j^\dagger\left[m_0\,\eta_3\Gamma_3\right]c_j \\ &+ g\sum_{j\neq k}\frac{F(r_{jk})}{2}c_j^\dagger\left[\cos(2\phi_{jk})\,\eta_0\Gamma_4\right]c_k + \Delta_{\rm FO}\sum_j c_j^\dagger\eta_1\sigma_1\tau_2 c_j + i\sum_j c_j^\dagger\left[\eta_0\Gamma_1 h_x + \eta_0\Gamma_2 h_y + \eta_0\Gamma_3 h_z\right]c_j, \end{aligned} \tag{S14}$$

which is the Nambu doubled version of Eq. (7) of the main text. The eight-component Nambu doubled spinor is defined as

$$c_j = \left[c_{j\uparrow\alpha}, c_{j\uparrow\beta}, c_{j\downarrow\alpha}, c_{j\downarrow\beta}, -ic^\dagger_{j\downarrow\alpha}, -ic^\dagger_{j\downarrow\beta}, ic^\dagger_{j\uparrow\alpha}, ic^\dagger_{j\uparrow\beta}\right]^\top. \tag{S15}$$

We numerically diagonalize the above Hamiltonian $H^{\rm pair}_{\rm SO}$ to arrive at the conclusions regarding the second-order Majorana skin effect, shown in the main text and Supplementary Information. For $h_z = 0$, the exact particle-hole symmetry of this model is generated by $\Theta^{\rm pair}_{\rm SO} = \eta_0\sigma_3\tau_1 {\rm I}_{\mathcal{A}}\mathcal{K}$.

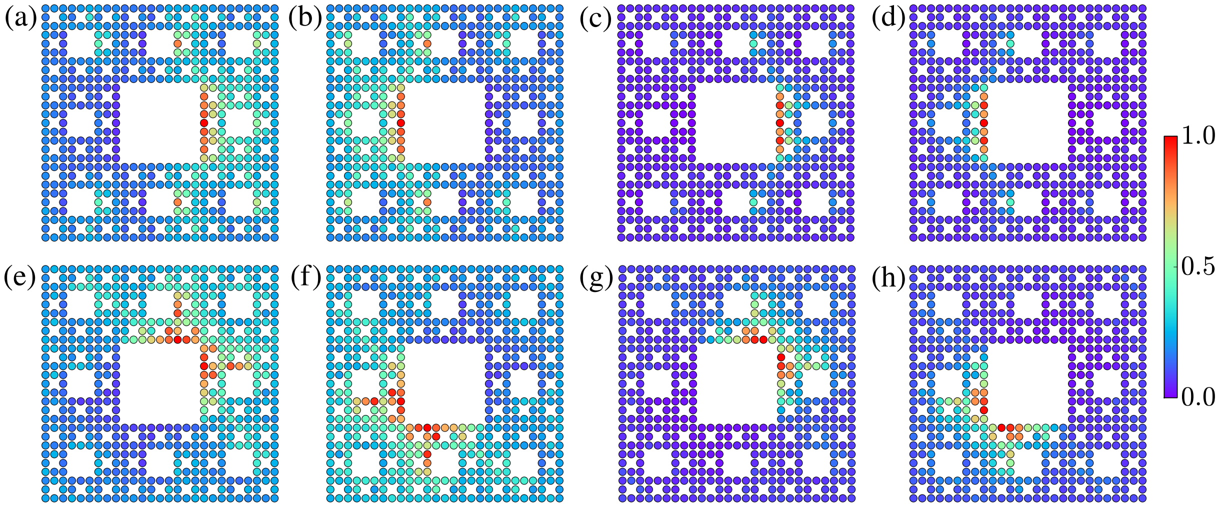


Supplementary Figure 9: First-order [(a)-(d)] and second-orer [(e)-(h)] inner skin effects for left [(a), (c), (e) and (g)] and right [(b), (d), (f) and (h)] eigenvectors. For (a) and (b), we choose $m_0 = -2.5$ and $h_x = 0.4$ in $H_{\rm FO}$, such that the NH Bott index $B_{\rm NH} = 0$ therein. For (c) and (d), we choose $m_0 = -0.5$ and $h_x = 1$ in $H_{\rm FO}$, such that $B_{\rm NH}$ is not well defined therein. For (e) and (f), we set $m_0 = 4.8$, $h_x = h_y = 0.53$ and $g = 0.5$ in $H_{\rm SO}$, such that that NH quadrupole moment $Q_{xy}^{\rm NH} = 0.0$ therein. For (g) and (h), we set $m_0 = 3.0$, $h_x = h_y = 1.0$ and $g = 0.5$ in $H_{\rm SO}$, such that $Q_{xy}^{\rm NH}$ is not well defined in this phase. Throughout we set $t = t_0 = 1$, $R = 2a$ and $r_0 = a$. See the phase diagrams in Fig. 3(d) and Fig. 4(c) of the main manuscript.

## Supplementary Note 5. ADDITIONAL NUMERICAL RESULTS

In the main manuscript, we presented ample numerical evidence to establish both first-order and second-order inner skin effects (ISEs) near the inner edges and corners, respectively, for charged and neutral Majorana fermions on two-dimensional Sierpinski carpet (SC) fractal lattices with periodic boundary conditions (PBCs), and contrasted these outcomes with ones on a square lattice, Ammann-Beenker (AB) quasicrystal and amorphous network, where skin effects only show up at the outer boundaries of these systems with open boudary conditions (OBCs). In this section of the Supplementary Information (SI), we present additional numerical results to support this claim. They are summarized in Supplementary Figure 1-Supplementary Figure 8. Below we present a brief description of these results.

In Supplementary Figure 1, we show the total normalized weight of all the right eigenvectors of $H_{\rm FO}$ on square lattice, AB quasicrystals, amorphous network and SC fractal lattice with OBC (top row) and PBC (bottom row). All four systems show NH skin effect at the outer right edge for the NH coupling $h_x$ with OBC. But, in systems with PBC in the $x$ direction only (a necessary and sufficient condition), the SC fractal lattice displays skin effect at the inner right edges, while the other three systems are devoid of any skin effect.

Supplementary Figure 2 displays total normalized weight of all the left (first and second rows) and right (thrid and fourth rows) eigenvectors of $H_{\rm FO}$ with OBCs (first and third rows) and PBCs (second and fourth rows) with NH coupling $h_x$ after performing average over 250 (first column), 500 (second column), 750 (third column) and 1000 (fourth column) random and independent realizations of 600 lattice points, constituting the amorphous network. With OBCs, the left and right eigenvectors respectively display clear signatures of the NH skin effect at the left and right edges of the amorphous network, irrespective of the number of site realizations. By contrast, the weight of both left and right eigenvectors are visibly uniform in the entire system, once we perform average over a sufficiently large number of site realizations, suggesting the absence of any skin effect even on amorphous network with PBCs.

We devote Supplementary Figure 3 to quantify and contrast (possible) skin effect on amorphous network. For this purpose, we devide the entire square-shaped network into sixteen bins, each of which is square in shape [panel (a)]. Then we compute the average standard deviation for the normalized weight of all the left eigenvectors in each bean

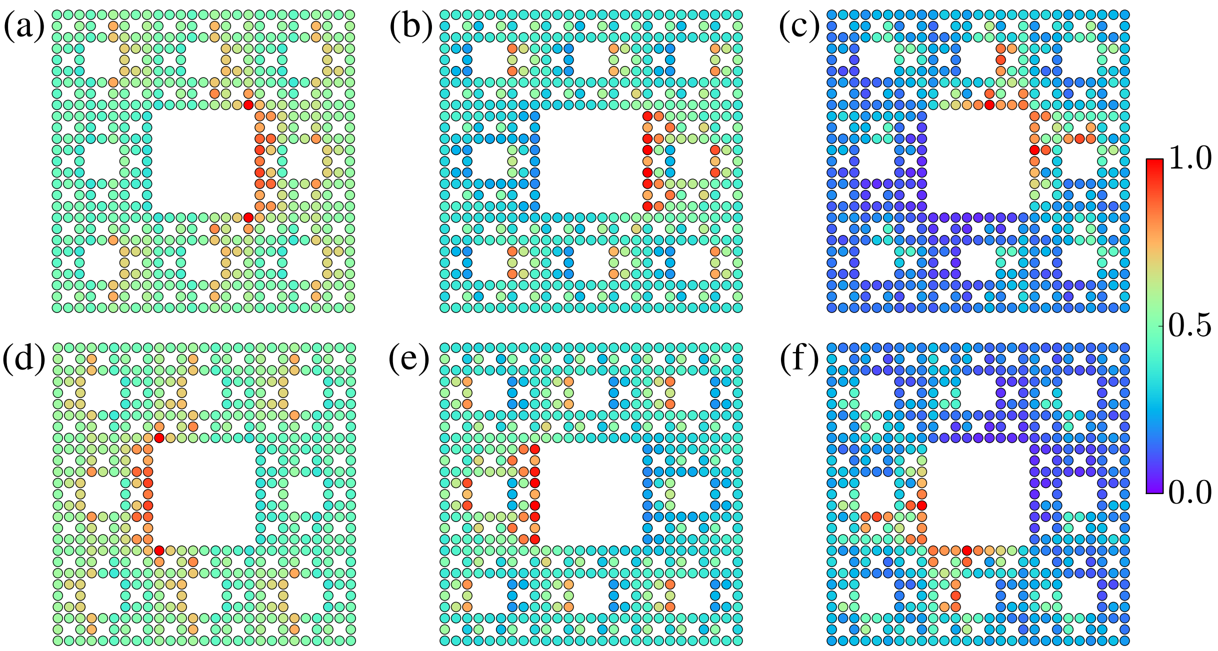


Supplementary Figure 10: First-order [(a), (b), (d) and (e)] and second-orer [(c) and (f)] Majorana inner skin effects for left [top row] and right [bottom row] eigenvectors. For (a) and (d), we choose $m_0 = 0.55$, $h_x = 0.5$, and $\Delta_{\rm FO} = 0.25$ in $H^{\rm pair}_{\rm FO}$, such that the NH Bott index $B_{\rm NH} = -2$ therein. For (b) and (e), we choose $m_0 = -4.5$, $h_x = 3.0$, and $\Delta_{\rm FO} = 0.25$ in $H^{\rm pair}_{\rm FO}$, such that $B_{\rm NH} = 0$ therein. For (c) and (f), we set $m_0 = -4.5$, $h_x = h_y = 1.0$, $g = 0.5$, and $\Delta_{\rm SO} = 0.025$ in $H^{\rm pair}_{\rm SO}$, such that that NH quadrupole moment $Q^{\rm NH}_{xy} = 0.0$ therein. Throughout we set $t = t_0 = 1$, $R = 2a$ and $r_0 = a$. See the phase diagrams in Fig. 4(b) and Fig. 4(d) of the main manuscript.

($\sigma$), defined as

$$\sigma = \frac{1}{M}\sum_{j=1}^{M} \sigma_j, \quad \text{where} \quad \sigma_j = \sqrt{\frac{1}{N}\sum_{i=1}^{N} (x_i(j) - \bar{x})^2} \tag{S16}$$

as a function of the bin number $b_N = 1, \cdots, 16$, for $N = 250$, 500, 750 and 1000 random and independent realizations of 600 sites constituting the amorphous network. Here $x_i(j)$ is the density of the left eigenvector at site $j$ in a given bin (containing total $M$ sites) for a given realization ($i$), and $\bar{x}$ is the average density of the left eigenvector in the entire network. With OBCs, $\sigma$ shows a clear peaks around the left edges of the systems for $b_N = 1, \cdots, 4$, in comparison to that in the rest of the system, bearing signatures of the NH skin effects therein. But, with PBC, $\sigma$ is *almost* uniform in the entire system, strongly suggesting absence of any skin effect on amorphous network with PBC. Also notice that for $N \geq 250$, $\sigma$ is independent of $N$ in the entire system irrespective of the nature of the boundary conditions.

Supplementary Figure 4 is analog to Fig. 3 of the main manuscript, however, with now PBCs in both $x$ and $y$ directions. We then show the spectra of $H_{\rm FO}$ in (a) a NH Chern insulator with NH Bott index $B_{\rm NH} = -1$, (b) a trivial insulator with $B_{\rm NH} = 0$ and (c) a NH insulator where $B_{\rm NH}$ is not well defined. As in Fig. 3 of the main text, the energy spectra in panels (a) and (b) display line gaps, while that in (c) show a point gap. In a NH Chern insulator phase, we now can only find the topological modes residing at the inner edges of the SC fractal lattice [black dots in panel (a)]. The resulting phase diagram [panel (d)], however, remains the same, as we previous obtained with PBC only in the $x$ direction. In panels (e) and (h) of Supplementary Figure 4, we show that the left eigenvectors of the states shown in black respectively in Fig. 3(a) of main manuscript and Supplementary Figure 4(a) with PBC in the $x$ direction and both $x$ and $y$ directions are localized in the inner left edges of the system. By contrast, the states shown as blue dots in Fig. 3(a) of the main manuscript appear at the bottom and top edges of system with PBC only in the $x$ direction, as shown in Supplementary Figure 4(f) and (g) from the density of the corresponding left eigenvectors. These states disappear with PBCs in both $x$ and $y$ directions. In each case, the corresponding right eigenvector appears at the opposite edge (outer or inner) of the system.

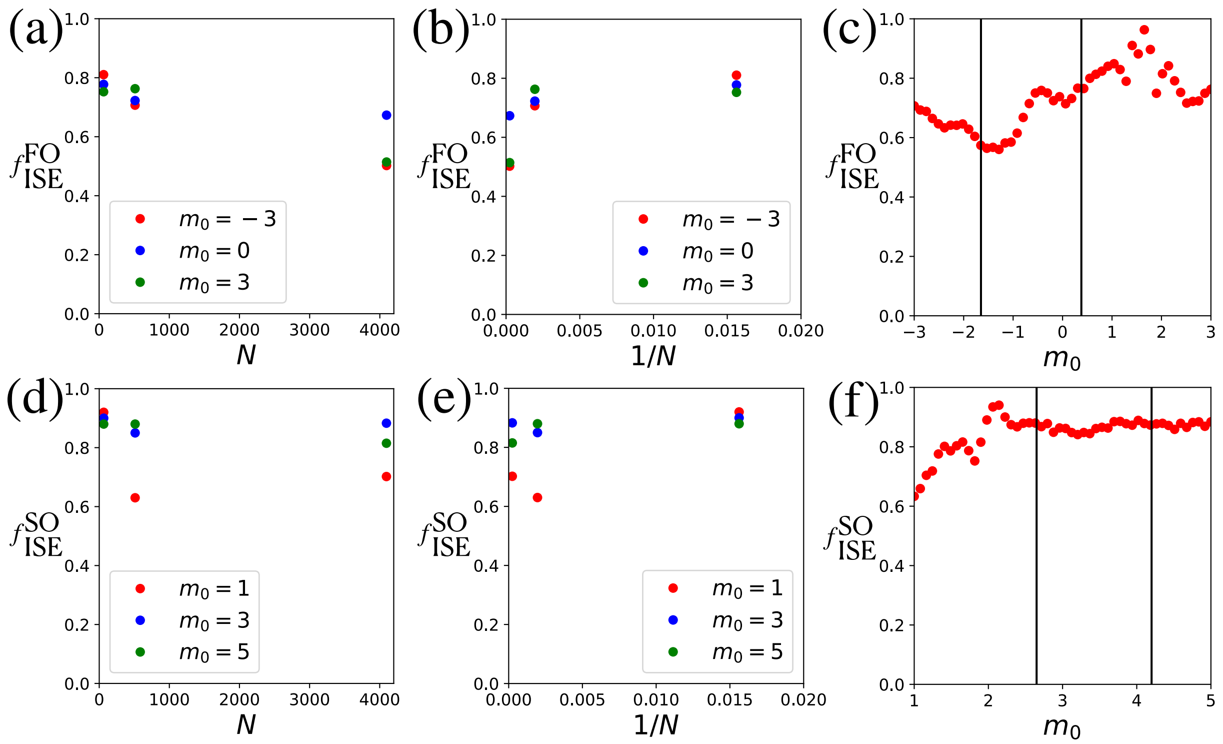


Supplementary Figure 11: Scaling of the fraction of the weight of all the states accumulated at the innermost edge of the Sierpinski carpet fractal, denoted by $f_{\rm ISE}^{\rm FO}$ that quantifies the first-order ISE, with (a) $N$ and (b) $1/N$, where $N$ is the total number of sites in a given generation. Here the results are shown for the first three generations, respectively containing 64, 512 and 4096 sites, showing that the ISE survives in the thermodynamic limit as $N \to \infty$ [see panel (b)]. Here the results are shown with $t = t_0 = 1$, $r_0 = a$, $R = 2a$, where $a$ is the nearest-neighbor distance and $h_x = 1.2$, for which we realize a NH Chern insulator with $B_{\rm NH} = -1$, trivial insulator with $B_{\rm NH} = 0$ and a NH insulator where $B_{\rm NH}$ is not well defined, respectively, for $m_0 = -3, 3$ and 0 [see Eq. (1) of the main manuscript]. (c) Scaling of $f_{\rm ISE}$ with the mass ($m_0$) for $h_x = 1.2$ on a Sierpinski carpet fractal of third generation, showing that it is always finite. The phase boundaries between distinct insulators are shown by vertical lines, near which $f_{\rm ISE}^{\rm FO}$ shows *weak* deeps as then the system becomes gapless. We arrive at the same conclusions for the left and right eigenvectors of $H_{\rm FO}$. These results remain qualitatively unchanged for any values of $m_0$ and $h_x$. Panels (d), (e) and (f) are similar to panels (a), (b) and (c), respectively, however quantifying second-order ISE in terms of $f_{\rm ISE}^{\rm SO}$. Here $f_{\rm ISO}^{\rm SO}$ measures the fraction of the weight of all the states accumulated near the innermost top-right corner of the Sierpinski carpet fractal. For the computation of $f_{\rm ISE}^{\rm SO}$ we take half of the innermost right and top edges as the top-right corner, since there is no site in the interior of the Sierpinski carpet fractal with only two nearest-neighbor sites, unlike the situation for the four outermost corners. Consequently, the second-order ISE spreads slightly away from the innermost top-right corner. Nonetheless, we find that $f_{\rm ISE}^{\rm SO}$ remains finite as the number of lattice sites in Sierpinski carpet fractal $N \to \infty$, as shown from the scaling of $f_{\rm ISE}^{\rm SO}$ with (d) $N$ and (e) $1/N$. In these two panels the results are shown for $t = t_0 = 1$, $r_0 = a$, $R = 2a$, $g = 0.5$ and $h_x = h_y = 0.5$, for which we realize NH quadrupole and trivial insulators with $Q_{xy}^{\rm NH} = 0.5$ and 0.0 respectively for $m_0 = 1$ and 5, and a NH insulator where $Q_{xy}^{\rm NH}$ is not well defined for $m_0 = 3$. In panel (f) we show $f_{\rm ISE}^{\rm SO}$ over a wide range of $m_0$ in a Sierpinski carpet fractal of second generation containing 512 sites, keeping all the parameters from panels (d) and (e) unchanged. It shows that in all the phases $f_{\rm ISE}^{\rm SO}$ remains finite, including at the phase boundaries between two topologically distinct insulators (marked by vertical lines). See Fig. 4(c) of the main manuscript for the phase diagram. We arrive at same conclusions for left and right eigenvectors of $H_{\rm SO}$ (see Eq. (4) of the main manuscript).

In Supplementary Figure 5, we show the second-order skin effect at the outer corner of a SC fractal lattice with OBCs in the $x$ and $y$ directions, and the second-order inner skin effect near the inner corners with PBCs in these two directions, however, for the right eigenvectors of $H_{\rm SO}$. When the second-order skin effect appears at the left-bottom corner of the SC fractal lattice with OBC, the corresponding inner skin effect appears near it left-bottom inner corners.

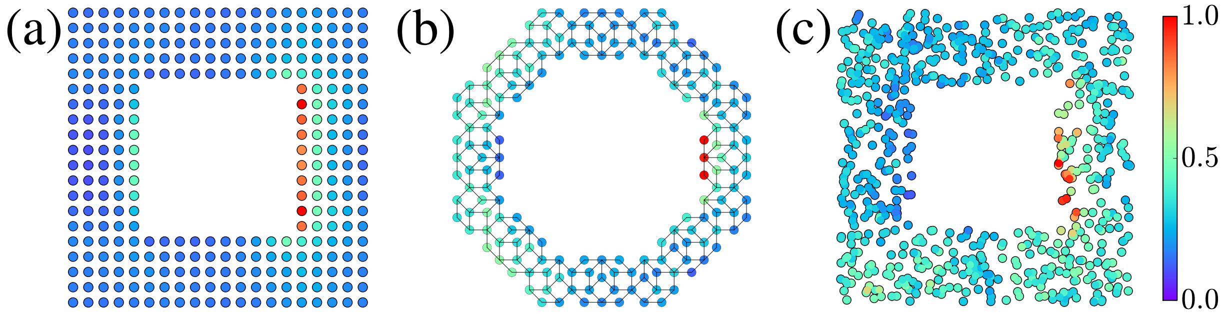


Supplementary Figure 12: First-order ISE on (a) square lattice, (b) Ammann-Beenker quasicrystal, and (c) amorphous network with a hollow region in the interior of the system, conforming to the Corbino geometry, and periodic boundary condition only in the horizontal $x$ direction. Here we show the normalized weight of all the left eigenvectors of $H_{\rm FO}$. Throughout we set $m_0 = 0$ and $t = t_0 = 1$ for all the systems. Here the results are shown for $\boldsymbol{h} = (0.4, 0, 0)$, $r_0 = a$ and $R = 2a$ [panels (a) and (b)] and $\boldsymbol{h} = (0.75, 0, 0)$, $r = 0.05a$ and $R = 0.10a$ [panel (c)]. In panel (a) [(b)] $a$ is the nearest-neighbor distance [the length of all the arms]. In panel (c) $a$ is the linear dimension of the system in both $x$ and $y$ directions. For the right eigenvectors of $H_{\rm FO}$ the ISE appears on the left interior edge of these systems. Note that the inner boundaries in these systems are artificially engineered from the outset, while the ones on fractal lattices stem from the intrinsic self-similarity symmetry.

The top panel of Supplementary Figure 6 shows first-order and second-order inner skin effects near the inner edges and corners, respectively, of the SC fractal lattices with PBCs in the $x$ direction and both $x$ and $y$ directions for neutral Majorana fermions, however, for the right eigenvectors of $H^{\rm pair}_{\rm FO}$ and $H^{\rm pair}_{\rm SO}$. The bottom panel of Supplementary Figure 6 shows the conventional first-order and second-order skin effect for neutral Majorana fermions at the outer edge and corner of the SC fractal lattices with OBCs, respectively. We arrive at qualitatively the same conclusions for both the left and right eigenvectors of $H^{\rm pair}_{\rm FO}$ and $H^{\rm pair}_{\rm SO}$.

The first-order NH skin effect at both inner and outer edges respectively with PBCs and OBCs are qualitatively insensitive to the generation number ($G_N$) of the SC fractal lattice, as explicitly shown for $G_N = 2$ (second generation) containing 64 lattice sites in Supplementary Figure 7 for normal or charged fermions. The same conclusions also hold for the second-order NH skin effect, where it shows up near the outer and inner corners of SC fractal lattice with OBC and PBC, respectively. The same outcomes are equally operative for neutral Majorana fermions, as shown in Supplementary Figure 8. In the main manuscript, we present these results on SC fractal lattice of third generation, containing 512 lattice sites.

In the main manuscript, we have shown both the first-order and second-order ISEs for charged and neutral Majorana fermions for the parameter values for which the corresponding NH topological invariants are nontrivial. Therefore, they correspond to intrinsic ISEs. However, ISEs are not tied with nonvanishing topological invariant. For example, first-order ISEs can be observed charged fermions when the NH Bott index $B_{\rm NH} = 0$ and when $B_{\rm NH}$ is not well defined (for strong NH couplings). On the other hand, second-order ISEs can be seen when the NH quadrupole moment $Q^{\rm NH}_{xy} = 0.0$ and when $Q^{\rm NH}_{xy}$ is not well defined (for strong NH couplings). These results are shown in Supplementary Figure 9. The similar conclusions hold for Majorana ISEs as well. For example, Majorana first-order ISEs are observed when $B_{\rm NH} = 0$ and $-2$. And Majorana second-order ISEs exist even when $Q^{\rm NH}_{xy} = 0.0$. These results are shown in Supplementary Figure 10.

The ISE, namely the first-order one, can be quantified from the scaling of the fraction of the weight of all the eigenvectors (left or right) of $H_{\rm FO}$ accumulated at the interiormost edge of the fractal lattice with PBC only along the horizontal $x$ direction, denoted by $f^{\rm FO}_{\rm ISE}$. The results summarized in Supplementary Figure 11 show that the ISEs remains finite as we approach the thermodynamic limit irrespective of the nature of the insulating states [panels (a) and (b)]. It also shows that while remaining finite in the entire phase diagram, near the phase boundary between distinct NH insulators $f^{\rm FO}_{\rm ISE}$ shows a weak deep [panel (c)], as the system becomes gapless there.

In the similar fashion, we also quantify the second-order ISE from the fraction of all the eigenvectors (left or right) of $H_{\rm SO}$ accumulated at the innermost top-right corner of the Sierpinski carpet fractal lattice with PBC in both the $x$ and $y$ directions, denoted by $f^{\rm FO}_{\rm ISE}$. The results are summarized in Supplementary Figure 11, show-

ing that $f_{\rm ISE}^{\rm FO}$ remains finite in the thermodynamic limit [panels (d) and (e)], and in the entire phase diagram [panel (f)].

Finally, we note that when a hollow region is created externally on a square lattice, amorphous network and quasicrystals, such systems can also display at least first-order ISE at the inner edges when periodic boundary condition only along the horizontal $x$ direction is imposed, as shown in Supplementary Figure 12. However, it must be noted that such inner boundaries are not intrinsic geometric property of these systems, rather engineered artificially from the outset, unlike the situation on fractal lattices.

## Supplementary References

[1] Bernevig, B. A., Hughes, T. L. & Zhang, S.-C. Quantum Spin Hall Effect and Topological Phase Transition in HgTe Quantum Wells, *Science* **314**, 1757 (2006).
[2] Manna, S., Nandy, S. & Roy, B. Higher-order topological phases on fractal lattices, *Phys. Rev. B* **105**, L201301 (2022).
[3] Benalcazar, W. A., Bernevig, B. A. & Hughes, T. L. Quantized electric multipole insulators, *Science* **357**, 61 (2017).
[4] Roy, B. Antiunitary symmetry protected higher-order topological phases, *Phys. Rev. Research* **1**, 032048(R) (2019).
[5] Roy, B. Higher-order topological superconductors in $\mathcal{P}$-, $\mathcal{T}$-odd quadrupolar Dirac materials, *Phys. Rev. B* **101**, 220506(R) (2020).
